# Supplementary material for: Unphysical and Physical Solutions in Many-Body Theories: from Weak to Strong Correlation
Source: arXiv:1503.07742 ancillary file (2015-04-21)
Supplement: Supplementary file 1 [file suppmat.pdf]

# Supplemental material for "Unphysical and Physical Solutions in Many-Body Theories: from Weak to Strong Correlation"

Adrian Stan,[1,2,3] Pina Romaniello,[4] Santiago Rigamonti,[5] Lucia Reining,[3] and J. A. Berger[6]

[1] *Sorbonne Universités, UPMC Université Paris VI, UMR8112, LERMA, F-75005, Paris, France*
[2] *LERMA, Observatoire de Paris, PSL Research University, CNRS, UMR8112, F-75014, Paris, France*
[3] *Laboratoire des Solides Irradiés, École Polytechnique, CNRS, CEA-DSM and European Theoretical Spectroscopy Facility (ETSF), 91128 Palaiseau, France*
[4] *Laboratoire de Physique Théorique, CNRS, IRSAMC, Université Toulouse III - Paul Sabatier and European Theoretical Spectroscopy Facility (ETSF), 118 Route de Narbonne, 31062 Toulouse Cedex, France*
[5] *Humboldt-Universität zu Berlin, Institut für Physik and IRIS Adlershof, and European Theoretical Spectroscopy Facility (ETSF), 12489 Berlin, Germany*
[6] *Laboratoire de Chimie et Physique Quantiques, IRSAMC, Université Toulouse III - Paul Sabatier, CNRS and European Theoretical Spectroscopy Facility (ETSF), 118 Route de Narbonne, 31062 Toulouse Cedex, France*

## CONVERGENCE PROBLEMS: THE EXAMPLE OF HARTREE FOCK

As an example of convergence problems in many-body theory we consider the Hartree-Fock (HF) approximation. The task is to solve the Dyson equation $G^{-1} = G_0^{-1} - \Sigma^{HF}[G]$. Usually this is done iteratively as, for example, $G^{-1(n+1)} = G_0^{-1} - \Sigma^{HF}[G^{(n)}]$. This iteration scheme can converge to a HF solution that is not necessarily the ground-state, or it can oscillate between two states, neither of which is a HF solution [1]. There are several approaches to overcome convergence problems (see Refs. [2–7]). For example, one can mix the results of previous iteration steps, as $G^{-1(n+1)} = G_0^{-1} - \Sigma[(1-\alpha)G^{(n)} + \alpha G^{(n-1)}]$, where $0 \leq \alpha \leq 1$ is the mixing parameter. In Fig. 1 we plot the HF total energy as a function of the interaction strength $U$ for a chain of ten sites with a Coulomb-like interaction $\gamma = Ue^{-0.5\,|i-j|}/|i-j|$ (with $i, j$ running over the sites). Without mixing ($\alpha = 0.0$) the HF total energy is linear in the interaction, but only for $U \leq 5$. For $U > 5$ the scheme oscillates between two values. Instead, using $\alpha = 0.5$ leads to a total energy that is linear in $U$ over a large range. In other words, this problem can be easily detected and solved. It does not appear in calculations that we have performed on Hubbard clusters, irrespective of the interaction strength.

## UNPHYSICAL SOLUTIONS IN TIME-DEPENDENT DENSITY-FUNCTIONAL THEORY

Optical absorption spectra can be obtained from the imaginary part of the macroscopic dielectric function $\epsilon_M$ that is related to the reducible polarizability $\chi$ according to

$$\epsilon_M(\omega) = 1/[1 + v_c\chi(\omega)]. \tag{1}$$

Here we neglected crystal local-field effects (LFE). The reducible polarizability $\chi(\omega)$ can be obtained from a Dyson-like equation:

$$\chi(\omega) = \chi_0(\omega) + \chi_0(\omega)\,[v_c + f_{xc}]\,\chi(\omega). \tag{2}$$

The bootstrap approximation to the exchange-correlation kernel $f_{xc}$ reads [8]:

$$f_{xc} = \frac{1 + v_c\chi(\omega = 0)}{\chi_0(\omega = 0)}. \tag{3}$$

This kernel is static by definition.

Since the bootstrap kernel depends on $\chi$, Eqs. (2) and (3) were solved iteratively in Ref. [8] (see also [9]). However, in Ref. [10] it was shown that these equations can be solved analytically and have two solutions, of which only one is physical. It turns out that the iteration scheme used in Ref. [8] gives the physical solution. Here we show that this iteration scheme is equivalent to scheme (**I**). Moreover, we show an iteration scheme, equivalent to scheme (**II**) that leads to well converged, but unphysical

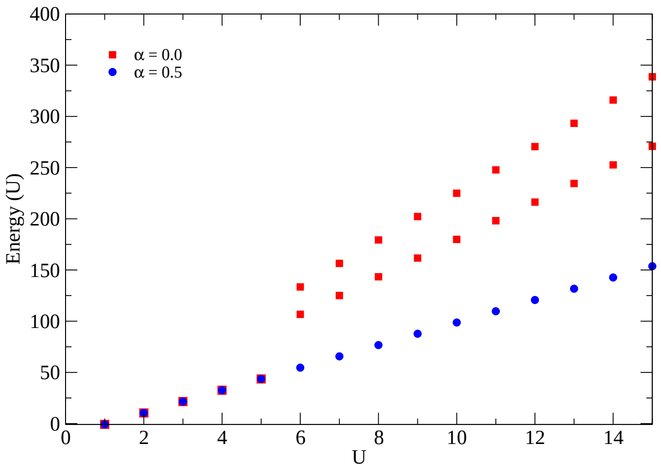


FIG. 1. (Color online) The Hartree-Fock (HF) total energy of a ten sites chain with a Coulomb-like interaction, as a function of the interaction $U$. Squares (red): results without mixing ($\alpha = 0.0$); circles (blue): results with mixing ($\alpha = 0.5$).

The analytical solution of the system of Eqs. (2) and (3) for $\omega = 0$ gives:

$$\chi^{\pm} = -\frac{\chi_0}{2} \pm \sqrt{\left(\frac{\chi_0}{2}\right)^2 - \frac{\chi_0}{v_c}} = -\frac{\chi_0}{2} \pm \left|\frac{\chi_0}{2}\right| \sqrt{1 - \frac{4}{v_c\chi_0}}. \tag{4}$$

The sign of the square root corresponding to the physical solution can be found by analyzing the limit of large screening $v_c\chi_0 \to -\infty$. For $\chi^-$, the correct result $\chi^- \to -1/v_c$, *i.e.*, the large screening random-phase approximation (RPA) result, is obtained. Note that in this limit, Eq.(3) also gives the expected RPA result, that is $f_{xc} = 0$. For $\chi^+$, the unphysical limit $\chi^+ \to -\chi_0$ is obtained. In practice, one would iterate Eqs.(2) and (3) up to self-consistency. Two iteration schemes emerge, which are given by setting $Y = -v_c\chi$ and $V = -2/v_c\chi_0$ in schemes (**I**) and (**II**). The physical solution is obtained using scheme (**I**), which is equivalent to the iterative solution proposed in [8].

If, instead of Eq.(2), the Dyson equation for the irreducible polarizability $P = \chi_0 + \chi_0 f_{xc} P$ is used, and the optical spectrum obtained from $\epsilon_M = 1 - v_c P$, one arrives again at schemes (**I**) and (**II**), with $Y = v_c P$ and $V = -2/v_c\chi_0$. In this case, however, the physical solution is given by scheme (**II**), which yields the correct large screening limit $P = \chi_0 \to -\infty$. This can be understood from the structure of the equations. It shows that the iteration scheme leading to the physical solution depends on the way in which the Dyson equation is formulated and that the OPM is a powerful tool to determine which iteration scheme has to be used.

*Ab initio* calculations of the optical spectrum of LiF were performed with the `exciting` code [11] using a grid of 4096 non-equivalent k-points. The LFE have been neglected. The Kohn-Sham eigenvalues from a ground-state calculation within the local-density approximation (LDA) (Perdew-Wang) [12] were corrected through a scissors shift of 5.22 eV in order to mimic the experimental quasiparticle gap $E_g^{\mathrm{LiF}} \approx 14.2$ eV [13].

## DEFINITION OF THE DOMAIN

Here we give an illustration for the restriction of the number of solutions for $G \to G_0$ to only one by restricting the domain of $G_0$ [14, 15]. Any physical Green's function should obey several physical constraints. For example, a physical $G_0$ can be expressed in its single-particle form,

$$G_0(x, x', \omega) = \sum_s \frac{\phi_s(x)\phi_s^*(x')}{\omega - \epsilon_s}, \tag{5}$$

where $\phi_s(x)$ and $\epsilon_s$ are the single-particle wave functions and energies, respectively. Let us now suppose that the Dyson equation given by

$$G_0^{-1} = G^{-1} + \Sigma[G]$$

with $G^{-1}$ fixed, has two solutions of the form (5), $G_0$ and $G_0'$. The difference of the two corresponding Dyson equations can be written as

$$[G_0']^{-1} = G_0^{-1} - \Sigma[G_0] + \Sigma[G_0']. \tag{6}$$

Now we write this equation in the basis labelled $\ell$ in which $G_0$ is diagonal. This basis exists and is the same for all frequencies because $G_0$ has the form given in Eq. (5). The right hand side of Eq. (6) in the basis reads $\delta_{\ell\ell'}(\omega - \epsilon_\ell) - \Sigma_{\ell\ell'}[G_0] + \Sigma_{\ell\ell'}[G_0']$. In the simple case of a static Hartree-Fock self-energy, this means that the off-diagonal elements of $[G_0']^{-1}$ must be static and therefore equal to their $\omega \to \infty$ limit. In this limit, for a spectrum $\epsilon_s$ that is bounded, these elements are zero and as a consequence $G_0'$ must be diagonal. This means that its wave functions are the same as those of $G_0$ and therefore $\Sigma_{HF}[G_0] = \Sigma_{HF}[G_0']$. We finally obtain that $G_0' = G_0$. We conclude that in this example the constraint (5) is sufficient to guarantee that there is only one solution. Hence, the problem of multiple solutions is related to the definition of the domain of representability of $G_0$.


[1] Cancès, Eric and Le Bris, Claude, ESAIM: M2AN **34**, 749 (2000).
[2] D. R. Hartree, *The calculation of atomic structures* (John Wiley and Sons, Inc., New York, 1957).
[3] V. R. Saunders and I. H. Hillier, Int. J. Quantum Chem. **7**, 699 (1973).
[4] P. Pulay, Chem. Phys. Lett. **73**, 393 (1980).
[5] P. Pulay, J. Comp. Chem. **3**, 556 (1982).
[6] E. Cancès and C. Le Bris, Int. J. Quantum Chem. **79**, 82 (2000).
[7] K. N. Kudin, G. E. Scuseria, and E. Cancès, J. Chem. Phys. **116**, 8255 (2002).
[8] S. Sharma, J. K. Dewhurst, A. Sanna, and E. K. U. Gross, Phys. Rev. Lett. **107**, 186401 (2011).
[9] The iterations are done only for $\omega = 0$.
[10] S. Rigamonti, S. Botti, V. Veniard, C. Draxl, L. Reining, and F. Sottile, Phys. Rev. Lett. **114**, 146402 (2015).
[11] A. Gulans, S. Kontur, C. Meisenbichler, D. Nabok, P. Pavone, S. Rigamonti, S. Sagmeister, U. Werner, and C. Draxl, Journal of Physics: Condensed Matter **26**, 363202 (2014).
[12] J. P. Perdew and Y. Wang, Phys. Rev. B **33**, 8800 (1986).
[13] M. Piacentini, D. W. Lynch, and C. G. Olson, Phys. Rev. B **13**, 5530 (1976).
[14] M. Potthoff, Eur. Phys. J. B **32**, 429 (2003).
[15] R. Eder, arXiv:1407.6599 (2014).
